# Supplementary material for: Spin-dependent (inverse) spin Hall effect in Co$_{60}$Fe$_{20}$B$_{20}$
Source: arXiv:1810.01227 ancillary file (2019-01-08)
Supplement: Supplementary file 1 [file supporting.pdf]

# Supporting Information

## Spin-dependent (inverse) spin Hall effect in $\text{Co}_{60}\text{Fe}_{20}\text{B}_{20}$

Joel Cramer,<sup>1,2</sup> Andrew Ross,<sup>1,2</sup> Lorenzo  
Baldrati,<sup>1</sup> Romain Lebrun,<sup>1</sup> and Mathias Kläui<sup>1,2,\*</sup>

<sup>1</sup>*Institute of Physics, Johannes Gutenberg-University Mainz, 55099 Mainz, Germany*

<sup>2</sup>*Graduate School of Excellence Materials Science in Mainz, 55128 Mainz, Germany*

## I. THERMALLY GENERATED VOLTAGES AS A FUNCTION OF FIELD

As discussed in the main text, non-local spin signals generated by thermal affects are not suitable to quantify the magnetization orientation-dependence of the spin-charge interconversion in  $\text{Co}_{60}\text{Fe}_{20}\text{B}_{20}$  (CoFeB). Nevertheless, such data can still be used to probe the magnetic characteristics of the investigated system. Figure. S1a, for instance, shows a  $V_{\Sigma}^{\text{nl}}$  hysteresis loop that has been obtained for the Pt  $\rightarrow$  CoFeB configuration and with the external magnetic field applied perpendicular to the wire ( $\alpha = 0^\circ, 180^\circ$ ). Apparently, the hysteresis loop reveals a complex multi level voltage switching. Regarding first the switching event at low fields (see inset), the comparison to the CoFeB  $\rightarrow$  Pt data shown in Fig. S1b signifies that this is attributable to the  $\text{Y}_3\text{Fe}_5\text{O}_{12}$  (YIG) magnetization reversal and thus the polarity inversion of the spin Seebeck effect (SSE) induced spin current.

In addition to the SSE reversal, a further evident feature of the hysteresis loop is a second switching event that occurs near  $-2$  mT and is only observed when sweeping the field from positive to negative values (sweep direction indicated by the colored arrows in the graph). The depth of this additional dip exhibits a roughly linear dependence on the applied heating power (see Fig. S2), signifying a thermal origin as for instance an anomalous Nernst effect (ANE) signal due to an additional out-of-plane gradient. The switching from a lower to a higher voltage level at  $-2$  mT implies that this additional thermal signal has a different sign than the SSE induced inverse spin Hall voltage, which is consistent with previous findings reported for  $\text{Co}_{20}\text{Fe}_{60}\text{B}_{20}$ <sup>1</sup>. The asymmetry of the switching, i.e., its exclusive appearance for one field sweep direction, may be due to the chosen wire structure or a localized defect breaking the inversion symmetry, potentially resulting in a unidirectional anisotropy. In the case of an incomplete capping of the CoFeB by the Ru layer, one possible mechanism one could think of would be a localized oxidation of the CoFeB leading to antiferromagnetic behavior and thus exchange bias<sup>2</sup>. Although the clarification of the origin of these features requires further studies, these findings clearly demonstrate that YIG and CoFeB are exchange decoupled by the Cu intermediate layer, as stated in the main text.

Apart from this aspect, the hysteresis in Fig. S1a shows a monotonic decrease of the voltage level for both field directions with increasing field amplitude, with the signal eventually saturating. Reconsidering the field dependence of  $\Delta\rho/\rho_0$  in Fig. 3 in the main text, this behavior is attributable to the CoFeB magnetization aligning along the field such that a supplementary thermal signal emerges or disappears. Since the total voltage change  $\Delta V_{\Sigma}$  has the same sign for both field directions, the additional signal can neither be provided by the ANE<sup>1</sup> nor a spin-dependent ISHE, for which one would expect asymmetric behavior. As already discussed in the main text, the  $\sin(2\alpha)$  symmetry of the planar Nernst effect (PNE) yields a possible explanation for  $\Delta V_{\Sigma}^{\text{nl}}$ . At low external fields, the CoFeB magnetization aligns along the long edge of the nanowire due to shape anisotropy such that, in the presence of an in-plane temperature gradient, a finite PNE voltage appears. If one now increases the external field amplitude,  $\mathbf{M}_{\text{CoFeB}}$  becomes parallel to the field ( $\alpha = 0^\circ, 180^\circ$ ) and the PNE contribution vanishes.

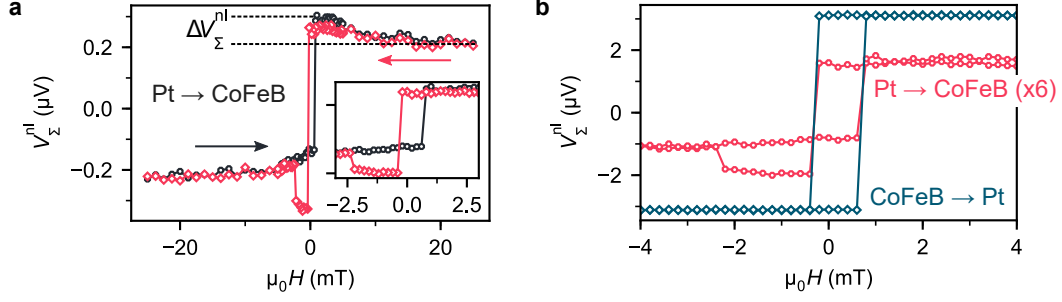

Figure S1. Thermal voltage hysteresis loops recorded for (a), (b) the Pt  $\rightarrow$  CoFeB and (b) the CoFeB  $\rightarrow$  Pt configuration. The external magnetic field is applied perpendicular to the wire. While the thermal signal at the Pt detector is induced by the spin Seebeck effect in YIG exclusively, additional anomalous and planar Nernst effect contributions may appear in the Pt  $\rightarrow$  CoFeB configuration. The arrows in (a) indicate the field sweep direction, while the inset shows a detailed scan at low fields. Beyond the displayed field range, the signals stay constant up to the maximum achievable field values of 185 mT.

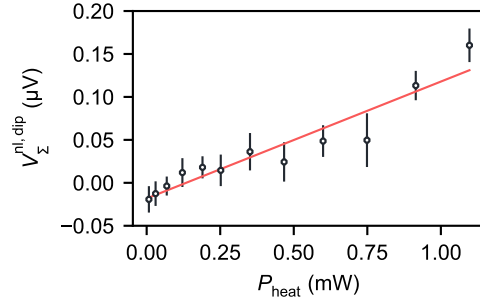

Figure S2. Height of the additional thermal voltage dip observed for the Pt  $\rightarrow$  CoFeB configuration when sweeping the field from positive to negative values, see Fig. S1a, as a function of the heating power applied to the Pt wire. The dip appears in the range of approximately  $-0.5$  mT to  $-2$  mT. The data can be described by a linear function. Error bars are given by propagated standard errors.

## II. FINITE ELEMENT SIMULATIONS OF OERSTED FIELD DISTRIBUTION IN THE CU/COFEB/RU NANOWIRE

Figure S3 shows the spatial variation of the generated Oersted field components when applying a charge current to the Cu/CoFeB/Ru nanowire to trigger spin currents. The results were obtained by performing a finite element simulation using the freely accessible software Agros2D<sup>3</sup>. The  $x$ - and  $y$ -components of the Oersted field just below and above the Cu/CoFeB interface are shown in Fig. S3a and Fig. S3b, respectively: blue solid lines give the field amplitude in the Cu layer, whereas red dashed line gives the field in the CoFeB. In the simulation, a total current of 300  $\mu$ A was applied to the wire. The current amplitudes flowing through the single Cu, CoFeB or Ru layers were estimated by considering the thicknesses and bulk/thin-film resistivities of the distinct layers ( $\rho_{\text{Cu}} = 1.7 \times 10^{-8} \Omega \text{ m}^4$ ,  $\rho_{\text{CoFeB}} = 2.3 \times 10^{-7} \Omega \text{ m}^5$ ,  $\rho_{\text{Ru}} = 7.1 \times 10^{-8} \Omega \text{ m}^4$ ). For the susceptibility, a value of  $\mu_r = 1000$  was chosen, which is of the order of magnitude for typical values reported for metallic ferromagnets<sup>4</sup>.

As discussed in the main text, the significant out-of-plane components of the Oersted field in the Cu layer may affect the polarization of the spin current due to an additional torque.

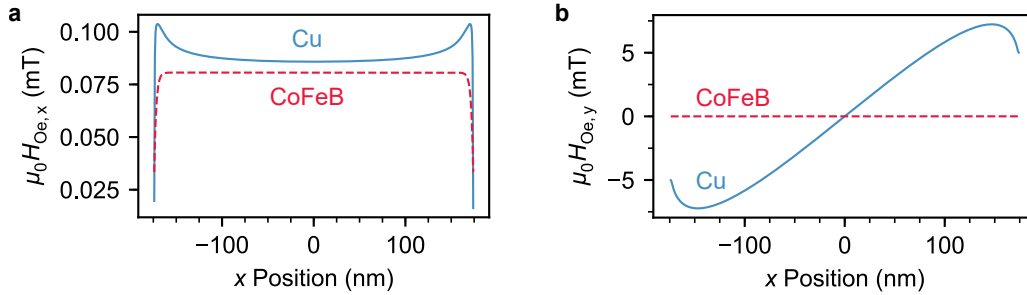

Figure S3. Spatial variation of the Oersted field generated in the Cu/CoFeB/Ru nanowire used to investigate the spin-dependent spin-charge interconversion in CoFeB. In (a) the  $x$ -component (in-plane, perpendicular to the long axis of the wire) is shown, while in (b) the  $y$ -component (out-of-plane) is given. Blue solid lines show the Oersted field in the Cu near the Cu/CoFeB interface, while the red dashed line shows the field in the CoFeB.

---

\* Klaeui@uni-mainz.de

- <sup>1</sup> S. M. Wu, J. Hoffman, J. E. Pearson, and A. Bhattacharya, Appl. Phys. Lett. **105**, 092409 (2014).
- <sup>2</sup> K. Gandha, R. P. Chaudhary, J. Mohapatra, A. R. Koymen, and J. P. Liu, Phys. Lett. A **381**, 2092 (2017).
- <sup>3</sup> Karban, P., Mach, F., Kůs, P., Pánek, D., Doležal, I. Numerical solution of coupled problems using code Agros2D. *Computing* **95**, 381-408 (2013).
- <sup>4</sup> W. M. Haynes, ed., *CRC handbook of chemistry and physics* (CRC press, 2005).
- <sup>5</sup> K. Seemann, F. Freimuth, H. Zhang, S. Blügel, Y. Mokrousov, D. Bürgler, and C. Schneider, Phys. Rev. Lett. **107**, 086603 (2011).
